# Supplementary material for: Unified treatment of synchronization patterns in generalized networks with higher-order, multilayer, and temporal interactions
Source: arXiv:2010.00613 ancillary file (2021-08-26)
Supplement: Supplementary file 1 [file SI.pdf]

# Supplementary Information

*Unified treatment of synchronization patterns in generalized networks with higher-order, multilayer, and temporal interactions*

Yuanzhao Zhang, Vito Latora, and Adilson E. Motter

## Supplementary Note 1. Variational equation for nonintertwined clusters in hypergraphs

The variational equation for a cluster synchronization pattern on a hypergraph has the following form:

$$\begin{aligned}\boldsymbol{\delta}_i[t+1] =& \mathrm{J}\boldsymbol{F}(\boldsymbol{s}^{m(i)})\boldsymbol{\delta}_i[t] + \sigma_1 \sum_j A_{ij}^{(1)} \left(\partial_{\boldsymbol{x}_i}\boldsymbol{H}^{(1)}(\boldsymbol{x}_i,\boldsymbol{x}_j)\,|_{\left(\boldsymbol{s}^{m(i)},\boldsymbol{s}^{m(j)}\right)}\boldsymbol{\delta}_i[t] + \partial_{\boldsymbol{x}_j}\boldsymbol{H}^{(1)}(\boldsymbol{x}_i,\boldsymbol{x}_j)\,|_{\left(\boldsymbol{s}^{m(i)},\boldsymbol{s}^{m(j)}\right)}\boldsymbol{\delta}_j[t]\right) \\ &+\sigma_2 \sum_{j,k} A_{ijk}^{(2)} \Big(\partial_{\boldsymbol{x}_i}\boldsymbol{H}^{(2)}(\boldsymbol{x}_i,\boldsymbol{x}_j,\boldsymbol{x}_k)\,|_{\left(\boldsymbol{s}^{m(i)},\boldsymbol{s}^{m(j)},\boldsymbol{s}^{m(k)}\right)}\boldsymbol{\delta}_i[t] + \partial_{\boldsymbol{x}_j}\boldsymbol{H}^{(2)}(\boldsymbol{x}_i,\boldsymbol{x}_j,\boldsymbol{x}_k)\,|_{\left(\boldsymbol{s}^{m(i)},\boldsymbol{s}^{m(j)},\boldsymbol{s}^{m(k)}\right)}\boldsymbol{\delta}_j[t] + \\ &\partial_{\boldsymbol{x}_k}\boldsymbol{H}^{(2)}(\boldsymbol{x}_i,\boldsymbol{x}_j,\boldsymbol{x}_k)\,|_{\left(\boldsymbol{s}^{m(i)},\boldsymbol{s}^{m(j)},\boldsymbol{s}^{m(k)}\right)}\boldsymbol{\delta}_k[t]\Big) + \sigma_3 \sum_{j,k,\ell} A_{ijk\ell}^{(3)} \cdots, \qquad i = 1,2,\dots,N,\end{aligned} \tag{S1}$$

where $m(i)$ denotes the cluster to which node $i$ belongs.

Since the clusters are not intertwined, each oscillator in the same cluster is affected by perturbations in other clusters in the same way [1, 2]. Thus, for all nodes $i$ that belong to a cluster $m$, the terms from Eq. (S1) involving $\boldsymbol{\delta}_j$ for $j \notin m$ can be combined into a single aggregated term $\boldsymbol{I}_m$. Moreover, each oscillator in cluster $m$ receives the same number of links $\mu_{m'\to m}$ from a different cluster $m'$. Using these conditions, the $\sigma_1$ term from Eq. (S1), which arise from the pairwise interactions, can be simplified to

$$\begin{aligned}&\sum_j A_{ij}^{(1)} \left(\partial_{\boldsymbol{x}_i}\boldsymbol{H}^{(1)}(\boldsymbol{x}_i,\boldsymbol{x}_j)\,|_{\left(\boldsymbol{s}^{m(i)},\boldsymbol{s}^{m(j)}\right)}\boldsymbol{\delta}_i[t] + \partial_{\boldsymbol{x}_j}\boldsymbol{H}^{(1)}(\boldsymbol{x}_i,\boldsymbol{x}_j)\,|_{\left(\boldsymbol{s}^{m(i)},\boldsymbol{s}^{m(j)}\right)}\boldsymbol{\delta}_j[t]\right) \\ =& \sum_{j\in m(i)} A_{ij}^{(1)} \left(\partial_{\boldsymbol{x}_i}\boldsymbol{H}^{(1)}(\boldsymbol{x}_i,\boldsymbol{x}_j)\,|_{\left(\boldsymbol{s}^{m(i)},\boldsymbol{s}^{m(i)}\right)}\boldsymbol{\delta}_i[t] + \partial_{\boldsymbol{x}_j}\boldsymbol{H}^{(1)}(\boldsymbol{x}_i,\boldsymbol{x}_j)\,|_{\left(\boldsymbol{s}^{m(i)},\boldsymbol{s}^{m(i)}\right)}\boldsymbol{\delta}_j[t]\right) + \\ &\sum_{j\notin m(i)} A_{ij}^{(1)} \left(\partial_{\boldsymbol{x}_i}\boldsymbol{H}^{(1)}(\boldsymbol{x}_i,\boldsymbol{x}_j)\,|_{\left(\boldsymbol{s}^{m(i)},\boldsymbol{s}^{m(j)}\right)}\boldsymbol{\delta}_i[t] + \partial_{\boldsymbol{x}_j}\boldsymbol{H}^{(1)}(\boldsymbol{x}_i,\boldsymbol{x}_j)\,|_{\left(\boldsymbol{s}^{m(i)},\boldsymbol{s}^{m(j)}\right)}\boldsymbol{\delta}_j[t]\right) \\ =& \sum_{j\in m(i)} A_{ij}^{(1)} \left(\partial_{\boldsymbol{x}_i}\boldsymbol{H}^{(1)}(\boldsymbol{x}_i,\boldsymbol{x}_j)\,|_{\left(\boldsymbol{s}^{m(i)},\boldsymbol{s}^{m(i)}\right)}\boldsymbol{\delta}_i[t] + \partial_{\boldsymbol{x}_j}\boldsymbol{H}^{(1)}(\boldsymbol{x}_i,\boldsymbol{x}_j)\,|_{\left(\boldsymbol{s}^{m(i)},\boldsymbol{s}^{m(i)}\right)}\boldsymbol{\delta}_j[t]\right) + \\ &\sum_{m'\neq m(i)} \mu_{m'\to m(i)}\partial_{\boldsymbol{x}_i}\boldsymbol{H}^{(1)}(\boldsymbol{x}_i,\boldsymbol{x}_j)\,|_{\left(\boldsymbol{s}^{m(i)},\boldsymbol{s}^{m'}\right)}\boldsymbol{\delta}_i[t] + \boldsymbol{I}_{m(i)}^{(1)}[t].\end{aligned} \tag{S2}$$

Since $\boldsymbol{H}^{(1)}(\boldsymbol{s},\boldsymbol{s}) = 0$ implies $\partial_{\boldsymbol{x}_i}\boldsymbol{H}^{(1)}(\boldsymbol{x}_i,\boldsymbol{x}_j)\,|_{(\boldsymbol{s},\boldsymbol{s})} = -\partial_{\boldsymbol{x}_j}\boldsymbol{H}^{(1)}(\boldsymbol{x}_i,\boldsymbol{x}_j)\,|_{(\boldsymbol{s},\boldsymbol{s})}$, it follows that the first r.h.s. term in Eq. (S2) can be expressed using the generalized Laplacian $\boldsymbol{L}^{(1)}$ as

$$-\sum_{j\in m(i)} L_{ij}^{(1)}\partial_{\boldsymbol{x}_j}\boldsymbol{H}^{(1)}(\boldsymbol{x}_i,\boldsymbol{x}_j)\,|_{\left(\boldsymbol{s}^{m(i)},\boldsymbol{s}^{m(i)}\right)}\boldsymbol{\delta}_j[t], \tag{S3}$$

where the diagonal entries in the generalized Laplacian only count the number of intracluster connections. The second and the third r.h.s. terms can be expressed using the diagonal matrices $\boldsymbol{D}^{(m)}$, since they both are equal for all nodes within a cluster.

Similarly, for three-body interactions, the corresponding term from Eq. (S1) can be simplified as follows:

$$\begin{aligned}
&\sum_{j,k} A_{ijk}^{(2)}\Big(\partial_{\boldsymbol{x}_i}\boldsymbol{H}^{(2)}\left(\boldsymbol{x}_i,\boldsymbol{x}_j,\boldsymbol{x}_k\right)|_{\left(\boldsymbol{s}^{m(i)},\boldsymbol{s}^{m(j)},\boldsymbol{s}^{m(k)}\right)}\boldsymbol{\delta}_i[t]+\partial_{\boldsymbol{x}_j}\boldsymbol{H}^{(2)}\left(\boldsymbol{x}_i,\boldsymbol{x}_j,\boldsymbol{x}_k\right)|_{\left(\boldsymbol{s}^{m(i)},\boldsymbol{s}^{m(j)},\boldsymbol{s}^{m(k)}\right)}\boldsymbol{\delta}_j[t]+\\
&\partial_{\boldsymbol{x}_k}\boldsymbol{H}^{(2)}\left(\boldsymbol{x}_i,\boldsymbol{x}_j,\boldsymbol{x}_k\right)|_{\left(\boldsymbol{s}^{m(i)},\boldsymbol{s}^{m(j)},\boldsymbol{s}^{m(k)}\right)}\boldsymbol{\delta}_k[t]\Big)\\
=&\sum_{j\in m(i),k\in m(i)} A_{ijk}^{(2)}\Big(\partial_{\boldsymbol{x}_i}\boldsymbol{H}^{(2)}\left(\boldsymbol{x}_i,\boldsymbol{x}_j,\boldsymbol{x}_k\right)|_{\left(\boldsymbol{s}^{m(i)},\boldsymbol{s}^{m(i)},\boldsymbol{s}^{m(i)}\right)}\boldsymbol{\delta}_i[t]+\partial_{\boldsymbol{x}_j}\boldsymbol{H}^{(2)}\left(\boldsymbol{x}_i,\boldsymbol{x}_j,\boldsymbol{x}_k\right)|_{\left(\boldsymbol{s}^{m(i)},\boldsymbol{s}^{m(i)},\boldsymbol{s}^{m(i)}\right)}\boldsymbol{\delta}_j[t]+\\
&\partial_{\boldsymbol{x}_k}\boldsymbol{H}^{(2)}\left(\boldsymbol{x}_i,\boldsymbol{x}_j,\boldsymbol{x}_k\right)|_{\left(\boldsymbol{s}^{m(i)},\boldsymbol{s}^{m(i)},\boldsymbol{s}^{m(i)}\right)}\boldsymbol{\delta}_k[t]\Big)+\\
&\sum_{j\notin m(i)|k\notin m(i)} A_{ijk}^{(2)}\Big(\partial_{\boldsymbol{x}_i}\boldsymbol{H}^{(2)}\left(\boldsymbol{x}_i,\boldsymbol{x}_j,\boldsymbol{x}_k\right)|_{\left(\boldsymbol{s}^{m(i)},\boldsymbol{s}^{m(j)},\boldsymbol{s}^{m(k)}\right)}\boldsymbol{\delta}_i[t]+\partial_{\boldsymbol{x}_j}\boldsymbol{H}^{(2)}\left(\boldsymbol{x}_i,\boldsymbol{x}_j,\boldsymbol{x}_k\right)|_{\left(\boldsymbol{s}^{m(i)},\boldsymbol{s}^{m(j)},\boldsymbol{s}^{m(k)}\right)}\boldsymbol{\delta}_j[t]+\\
&\partial_{\boldsymbol{x}_k}\boldsymbol{H}^{(2)}\left(\boldsymbol{x}_i,\boldsymbol{x}_j,\boldsymbol{x}_k\right)|_{\left(\boldsymbol{s}^{m(i)},\boldsymbol{s}^{m(j)},\boldsymbol{s}^{m(k)}\right)}\boldsymbol{\delta}_k[t]\Big)\\
=&\sum_{j\in m(i),k\in m(i)} A_{ijk}^{(2)}\Big(\partial_{\boldsymbol{x}_i}\boldsymbol{H}^{(2)}\left(\boldsymbol{x}_i,\boldsymbol{x}_j,\boldsymbol{x}_k\right)|_{\left(\boldsymbol{s}^{m(i)},\boldsymbol{s}^{m(i)},\boldsymbol{s}^{m(i)}\right)}\boldsymbol{\delta}_i[t]+\partial_{\boldsymbol{x}_j}\boldsymbol{H}^{(2)}\left(\boldsymbol{x}_i,\boldsymbol{x}_j,\boldsymbol{x}_k\right)|_{\left(\boldsymbol{s}^{m(i)},\boldsymbol{s}^{m(i)},\boldsymbol{s}^{m(i)}\right)}\boldsymbol{\delta}_j[t]+\\
&\partial_{\boldsymbol{x}_k}\boldsymbol{H}^{(2)}\left(\boldsymbol{x}_i,\boldsymbol{x}_j,\boldsymbol{x}_k\right)|_{\left(\boldsymbol{s}^{m(i)},\boldsymbol{s}^{m(i)},\boldsymbol{s}^{m(i)}\right)}\boldsymbol{\delta}_k[t]\Big)+\\
&\sum_{m'\neq m(i)|m''\neq m(i)} \mu_{m'm''\to m(i)}\partial_{\boldsymbol{x}_i}\boldsymbol{H}^{(2)}\left(\boldsymbol{x}_i,\boldsymbol{x}_j,\boldsymbol{x}_k\right)|_{\left(\boldsymbol{s}^{m(i)},\boldsymbol{s}^{m'},\boldsymbol{s}^{m''}\right)}\boldsymbol{\delta}_i[t]+\\
&\sum_{j\in m(i),m'\neq m(i)} \mu_{m'm(i)\to m(i)}\partial_{\boldsymbol{x}_j}\boldsymbol{H}^{(2)}\left(\boldsymbol{x}_i,\boldsymbol{x}_j,\boldsymbol{x}_k\right)|_{\left(\boldsymbol{s}^{m(i)},\boldsymbol{s}^{m(i)},\boldsymbol{s}^{m'}\right)}\boldsymbol{\delta}_j[t]+\\
&\sum_{k\in m(i),m'\neq m(i)} \mu_{m'm(i)\to m(i)}\partial_{\boldsymbol{x}_k}\boldsymbol{H}^{(2)}\left(\boldsymbol{x}_i,\boldsymbol{x}_j,\boldsymbol{x}_k\right)|_{\left(\boldsymbol{s}^{m(i)},\boldsymbol{s}^{m'},\boldsymbol{s}^{m(i)}\right)}\boldsymbol{\delta}_k[t]+\boldsymbol{I}_{m(i)}^{(2)}[t].
\end{aligned} \tag{S4}$$

Here, the $|$ symbol under $\sum$ denotes the logical OR operator and $\mu_{m'm''\to m}$ represents the number of three-body interactions a node in cluster $m$ receives that involve a node from cluster $m'$ and another node from cluster $m''$. Again, using the noninvasive property $\boldsymbol{H}^{(2)}(\boldsymbol{s},\boldsymbol{s},\boldsymbol{s})=0$, the first r.h.s. term in this equation can be expressed using the generalized Laplacian $\boldsymbol{L}^{(2)}$ as

$$-\sum_{j\in m(i)} L_{ij}^{(2)}\left(\partial_{\boldsymbol{x}_j}\boldsymbol{H}^{(2)}\left(\boldsymbol{x}_i,\boldsymbol{x}_j,\boldsymbol{x}_k\right)|_{\left(\boldsymbol{s}^{m(i)},\boldsymbol{s}^{m(i)},\boldsymbol{s}^{m(i)}\right)}+\partial_{\boldsymbol{x}_k}\boldsymbol{H}^{(2)}\left(\boldsymbol{x}_i,\boldsymbol{x}_j,\boldsymbol{x}_k\right)|_{\left(\boldsymbol{s}^{m(i)},\boldsymbol{s}^{m(i)},\boldsymbol{s}^{m(i)}\right)}\right)\boldsymbol{\delta}_j[t], \tag{S5}$$

where the entries in $\boldsymbol{L}^{(2)}$ only take into account the intracluster 2-simplices [3]. Similarly to the case of pairwise interactions, the other r.h.s. terms can be expressed using the diagonal matrices $\boldsymbol{D}^{(m)}$. The derivations above can be easily adapted to include higher-order interactions that involve more than three nodes simultaneously.

## Supplementary Note 2. Analytical condition for chimera stability

For the system in Fig. 2, $F(x)=\beta\sin^2\left(x+\pi/4\right)$, $H^{(1)}(x_i,x_j)=\sin^2\left(x_j+\pi/4\right)-\sin^2\left(x_i+\pi/4\right)$, and $H^{(2)}(x_i,x_j,x_k)=\sin^2\left(x_j+x_k-2x_i\right)$. According to Eq. (S1), the stability of the coherent subnetwork $C_1$ (and thus the stability of the chimera state) is determined by the following variational equation:

$$\begin{aligned}
\delta_i[t+1]=&\,\mathrm{J}F(s[t])\delta_i[t]+\sigma_1\sum_j A_{ij}^{(1)}\left(\partial_{x_i}H^{(1)}\left(x_i,x_j\right)|_{\left(s,s^{m(j)}\right)}\delta_i[t]+\partial_{x_j}H^{(1)}\left(x_i,x_j\right)|_{\left(s,s^{m(j)}\right)}\delta_j[t]\right)\\
&+\sigma_2\sum_{j,k}A_{ijk}^{(2)}\left(\partial_{x_i}H^{(2)}\left(x_i,x_j,x_k\right)|_{\left(s,s^{m(j)},s^{m(k)}\right)}\delta_i[t]+\partial_{x_j}H^{(2)}\left(x_i,x_j,x_k\right)|_{\left(s,s^{m(j)},s^{m(k)}\right)}\delta_j[t]+\right.\\
&\left.\partial_{x_k}H^{(2)}\left(x_i,x_j,x_k\right)|_{\left(s,s^{m(j)},s^{m(k)}\right)}\delta_k[t]\right),\qquad i\in C_1,
\end{aligned} \tag{S6}$$

where $s$ represents the synchronization trajectory in $C_1$. Since the clusters are not intertwined, from Eqs. (S2) and (S3) we know the pairwise interaction term

$$\begin{aligned}&\sum_j A_{ij}^{(1)}\left(\partial_{x_i}H^{(1)}(x_i,x_j)|_{\left(s,s^{m(j)}\right)}\delta_i[t]+\partial_{x_j}H^{(1)}(x_i,x_j)|_{\left(s,s^{m(j)}\right)}\delta_j[t]\right)\\&=-\sum_{j\in C_1}L_{ij}^{(1)}\partial_{x_j}H^{(1)}(x_i,x_j)|_{(s,s)}\delta_j[t]+\sum_{j\in C_2}\partial_{x_i}H^{(1)}(x_i,x_j)|_{\left(s,s^{m(j)}\right)}\delta_i[t]+I^{(1)}[t].\end{aligned}\tag{S7}$$

Moreover, since there are no three-body interactions between $C_1$ and $C_2$, the three-body interaction term simplifies to

$$\begin{aligned}&\sum_{j,k\in C_1}A_{ijk}^{(2)}\left(\partial_{x_i}H^{(2)}(x_i,x_j,x_k)|_{(s,s,s)}\delta_i[t]+\partial_{x_j}H^{(2)}(x_i,x_j,x_k)|_{(s,s,s)}\delta_j[t]+\partial_{x_k}H^{(2)}(x_i,x_j,x_k)|_{(s,s,s)}\delta_k[t]\right)\\&=-\sum_{j\in C_1}L_{ij}^{(2)}\left(\partial_{x_j}H^{(2)}(x_i,x_j,x_k)|_{(s,s,s)}+\partial_{x_k}H^{(2)}(x_i,x_j,x_k)|_{(s,s,s)}\right)\delta_j[t].\end{aligned}\tag{S8}$$

From the SBD algorithm, we know that the transverse blocks of $\{\boldsymbol{D}^{(1)},\cdots,\boldsymbol{D}^{(8)},\boldsymbol{L}^{(1)},\boldsymbol{L}^{(2)}\}$ are $1\times1$ (Fig. 2b). Thus, the decoupled variational equation corresponding to each transverse block has the following form

$$\begin{aligned}\eta_i[t+1]=&\Bigg\{\mathrm{J}F(s)-\sigma_1\lambda_i^{(1)}\partial_{x_j}H^{(1)}(x_i,x_j)|_{(s,s)}+\kappa\sigma_1\sum_{j\in C_2}\partial_{x_i}H^{(1)}(x_i,x_j)|_{\left(s,s^{m(j)}\right)}\\&-\sigma_2\lambda_i^{(2)}\left(\partial_{x_j}H^{(2)}(x_i,x_j,x_k)|_{(s,s,s)}+\partial_{x_k}H^{(2)}(x_i,x_j,x_k)|_{(s,s,s)}\right)\Bigg\}\eta_i[t].\end{aligned}\tag{S9}$$

Since $H^{(1)}(x_i,x_j)=\sin^2\left(x_j+\pi/4\right)-\sin^2\left(x_i+\pi/4\right)$, we have

$$\partial_{x_i}H^{(1)}(x_i,x_j)|_{\left(s,s^{m(j)}\right)}=-\partial_{x_j}H^{(1)}(x_i,x_j)|_{(s,s)}=-\frac{1}{\beta}\mathrm{J}F(s)=-2\sin\left(s+\pi/4\right)\cos\left(s+\pi/4\right)=-\sin\left(2s+\pi/2\right)\tag{S10}$$

regardless of the value of $j$. As a result,

$$\sum_{j\in C_2}\partial_{x_i}H^{(1)}(x_i,x_j)|_{\left(s,s^{m(j)}\right)}=-\frac{N}{2}\partial_{x_j}H^{(1)}(x_i,x_j)|_{(s,s)}=-\frac{N}{2}\frac{1}{\beta}\mathrm{J}F(s).\tag{S11}$$

Moreover, for $H^{(2)}(x_i,x_j,x_k)=\sin^2\left(x_j+x_k-2x_i\right)$, it is easy to verify that $\partial_{x_j}H^{(2)}(x_i,x_j,x_k)|_{(s,s,s)}=\partial_{x_k}H^{(2)}(x_i,x_j,x_k)|_{(s,s,s)}=0$. Thus, the decoupled variational equation (S9) can be further simplified into

$$\eta_i[t+1]=\left\{\mathrm{J}F(s)-\frac{\sigma_1}{\beta}\left(\lambda_i^{(1)}+\frac{\kappa N}{2}\right)\mathrm{J}F(s)\right\}\eta_i[t].\tag{S12}$$

The corresponding Lyapunov exponent $\Lambda_i$ can then be calculated as

$$\begin{aligned}\Lambda_i&=\lim_{\mathcal{T}\to\infty}\frac{1}{\mathcal{T}}\ln\left|\prod_{t=1}^{\mathcal{T}}\left(1-\frac{\sigma_1}{\beta}\left(\lambda_i^{(1)}+\frac{\kappa N}{2}\right)\right)\mathrm{J}F(s[t])\right|\\&=\lim_{\mathcal{T}\to\infty}\frac{1}{\mathcal{T}}\sum_{t=1}^{\mathcal{T}}\left\{\ln\left|1-\frac{\sigma_1}{\beta}\left(\lambda_i^{(1)}+\frac{\kappa N}{2}\right)\right|+\ln|\mathrm{J}F(s[t])|\right\}\\&=\ln\left|1-\frac{\sigma_1}{\beta}\left(\lambda_i^{(1)}+\frac{\kappa N}{2}\right)\right|+\lim_{\mathcal{T}\to\infty}\frac{1}{\mathcal{T}}\sum_{t=1}^{\mathcal{T}}\ln|\mathrm{J}F(s[t])|\\&=\ln\left|1-\frac{\sigma_1}{\beta}\left(\lambda_i^{(1)}+\frac{\kappa N}{2}\right)\right|+\Gamma.\end{aligned}\tag{S13}$$

---


[1] Pecora, L. M., Sorrentino, F., Hagerstrom, A. M., Murphy, T. E. & Roy, R. Cluster synchronization and isolated desynchronization in complex networks with symmetries. *Nat. Commun.* **5**, 4079 (2014).

[2] Cho, Y. S., Nishikawa, T. & Motter, A. E. Stable chimeras and independently synchronizable clusters. *Phys. Rev. Lett.* **119**, 084101 (2017).

[3] Gambuzza, L. *et al.* Stability of synchronization in simplicial complexes. *Nat. Commun.* **12**, 1255 (2021).
